# Supplementary material for: SoK: Liquid Staking Tokens (LSTs) and Emerging Trends in Restaking
Source: arXiv:2404.00644 source file (2024-12-26)
Supplement: Supplementary file 1 [file 99Appendix.tex]

\subsection{Additional Figures and Tables}
The following pages of this appendix contain supplementary figures.

\begin{figure*}[tbh]
  \begin{minipage}[c]{0.5\textwidth}
    \includegraphics[width=0.99\linewidth]{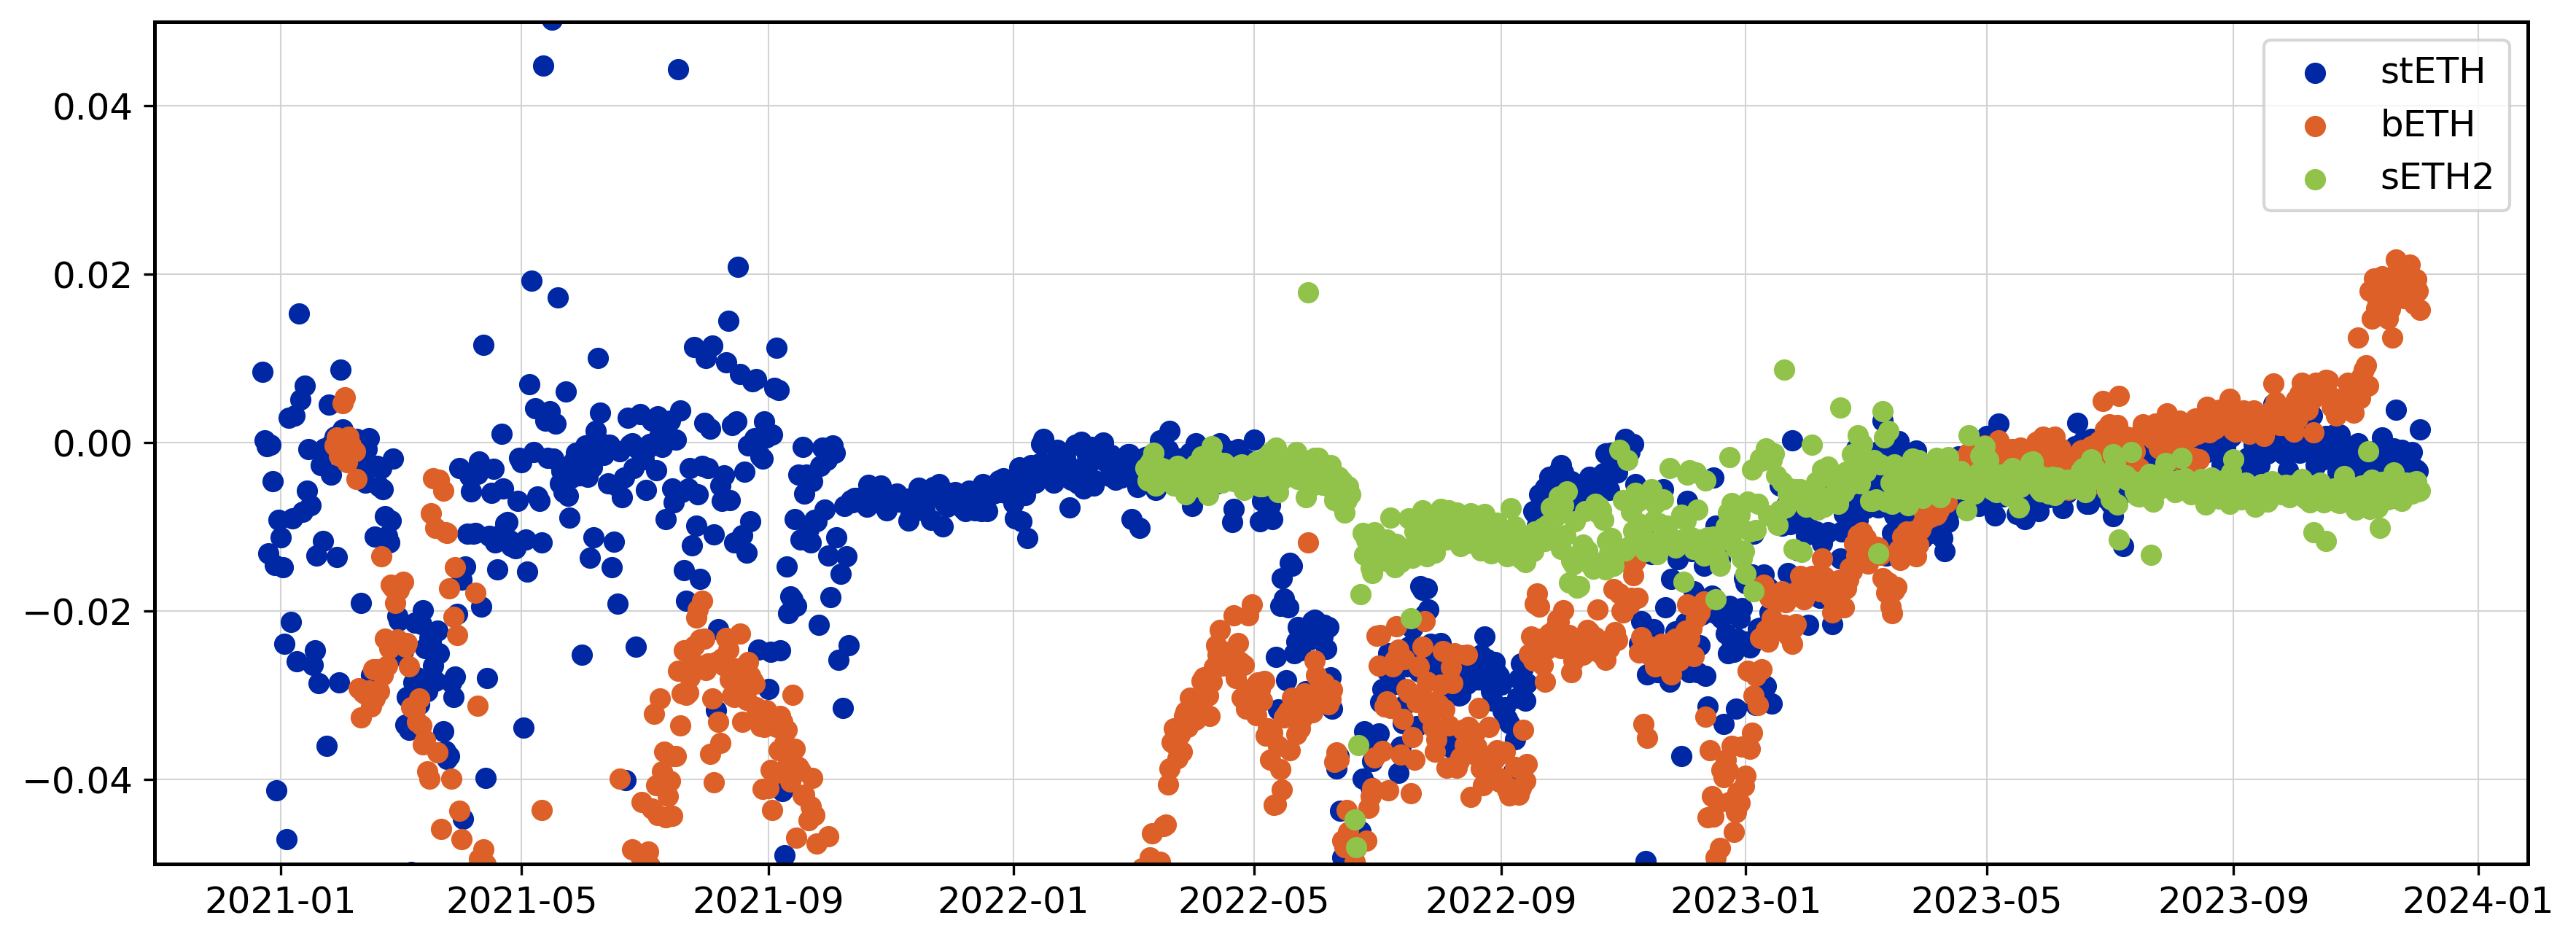} 
  \end{minipage} 
  \begin{minipage}[c]{0.5\textwidth}
    \includegraphics[width=.99\linewidth]{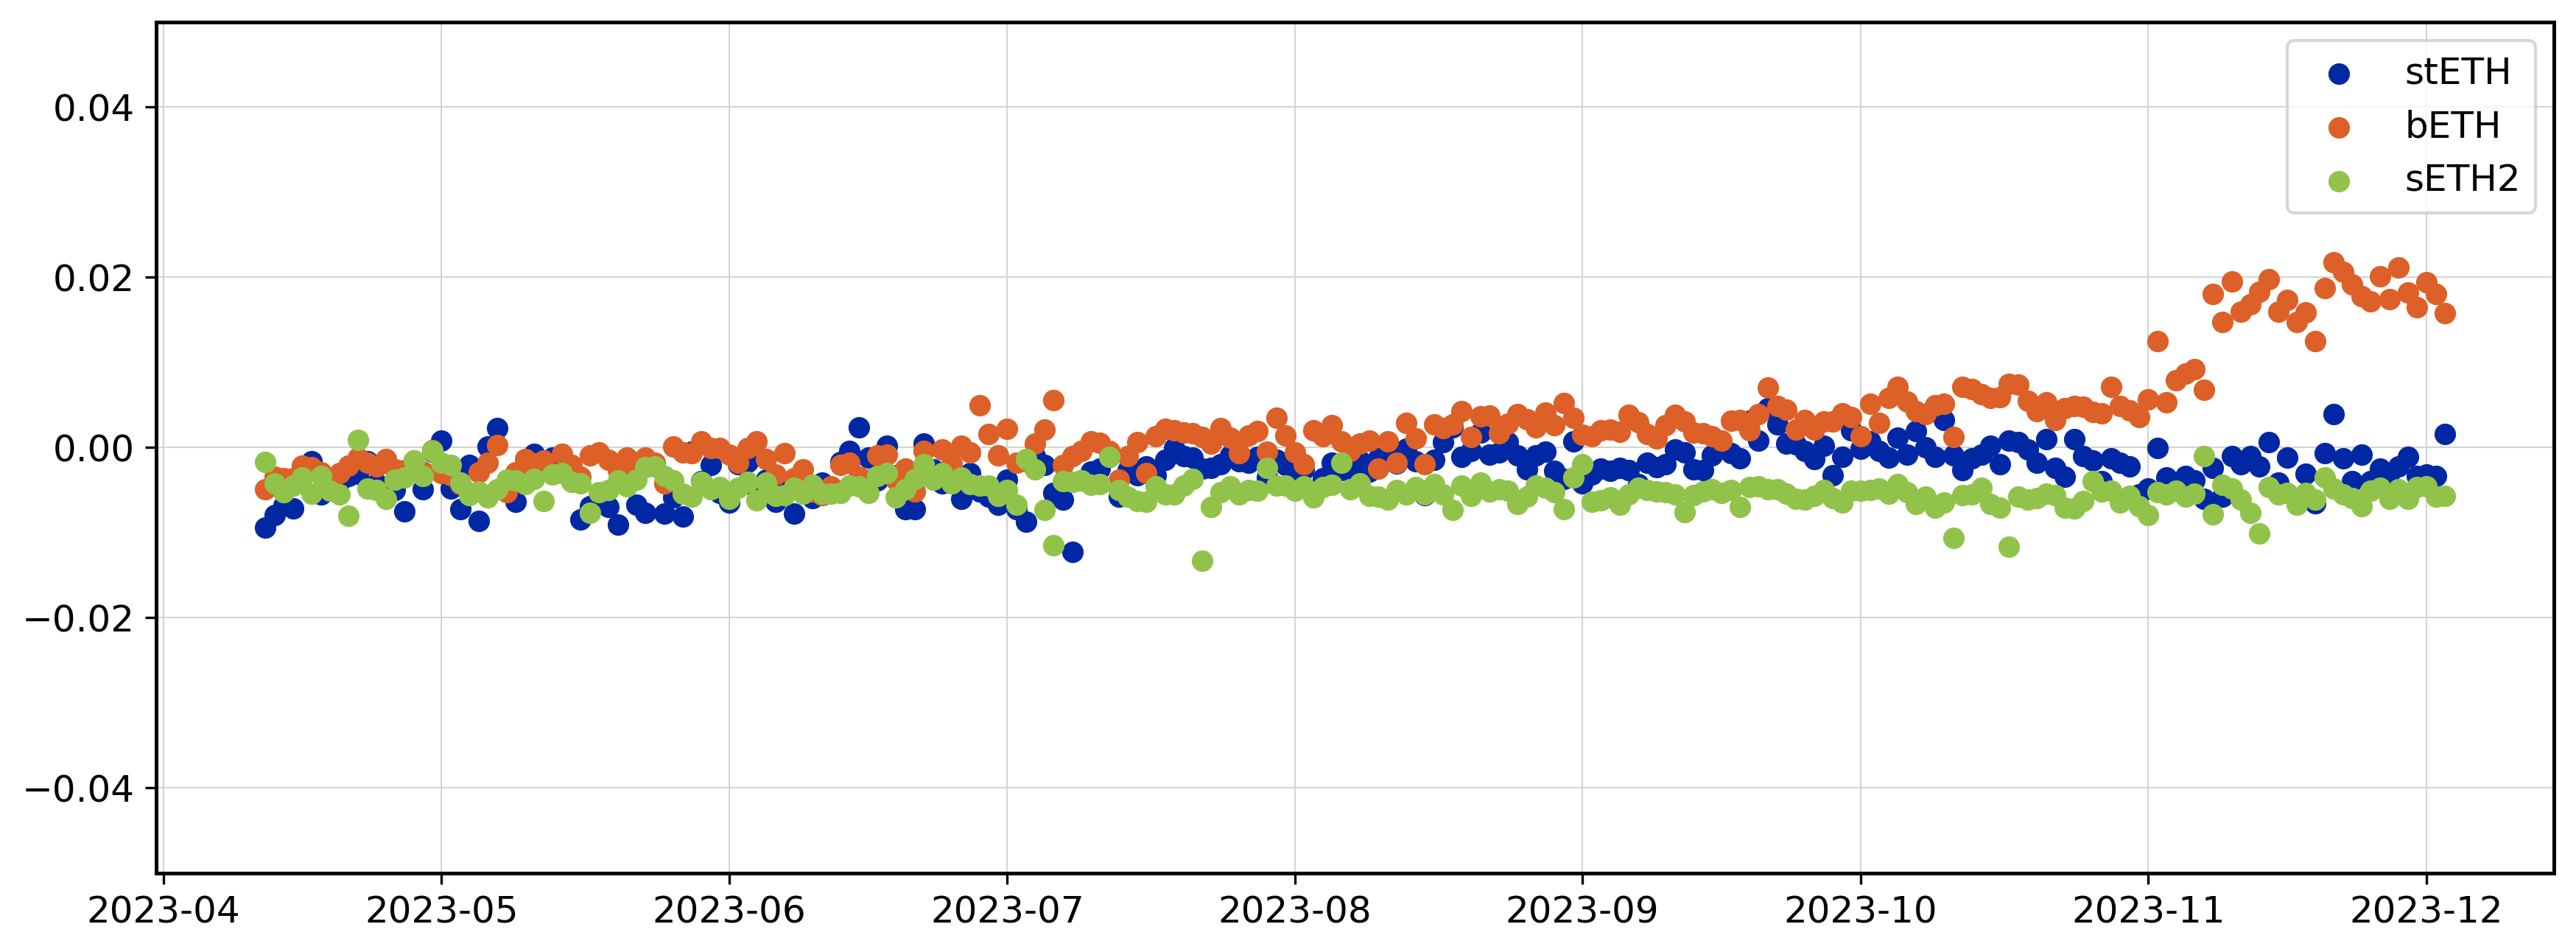} 
  \end{minipage} 
\hfill
    \begin{minipage}[c]{0.5\textwidth}
    \includegraphics[width=0.99\linewidth]{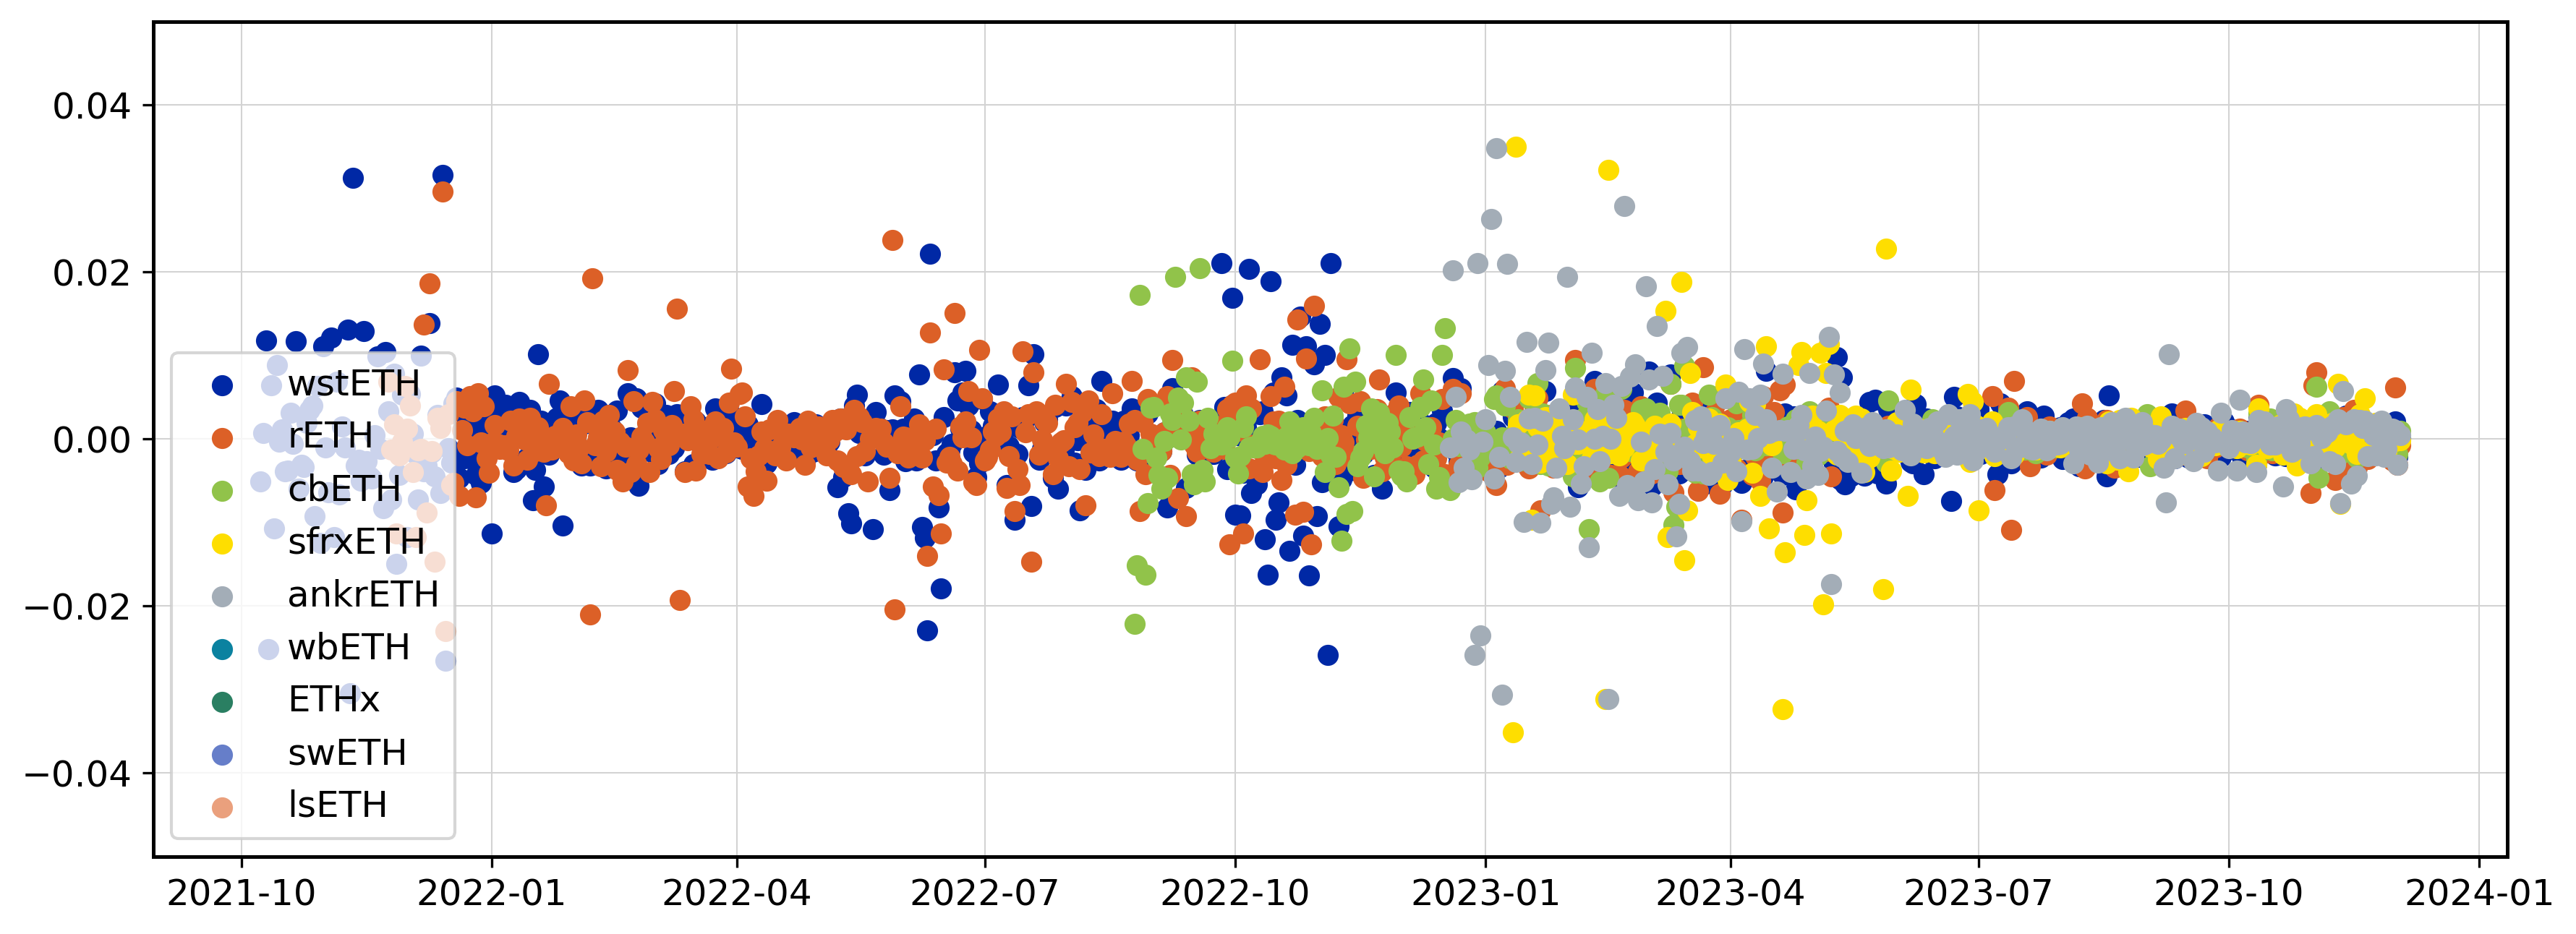} 
  \end{minipage} 
  \begin{minipage}[c]{0.5\textwidth}
    \includegraphics[width=.99\linewidth]{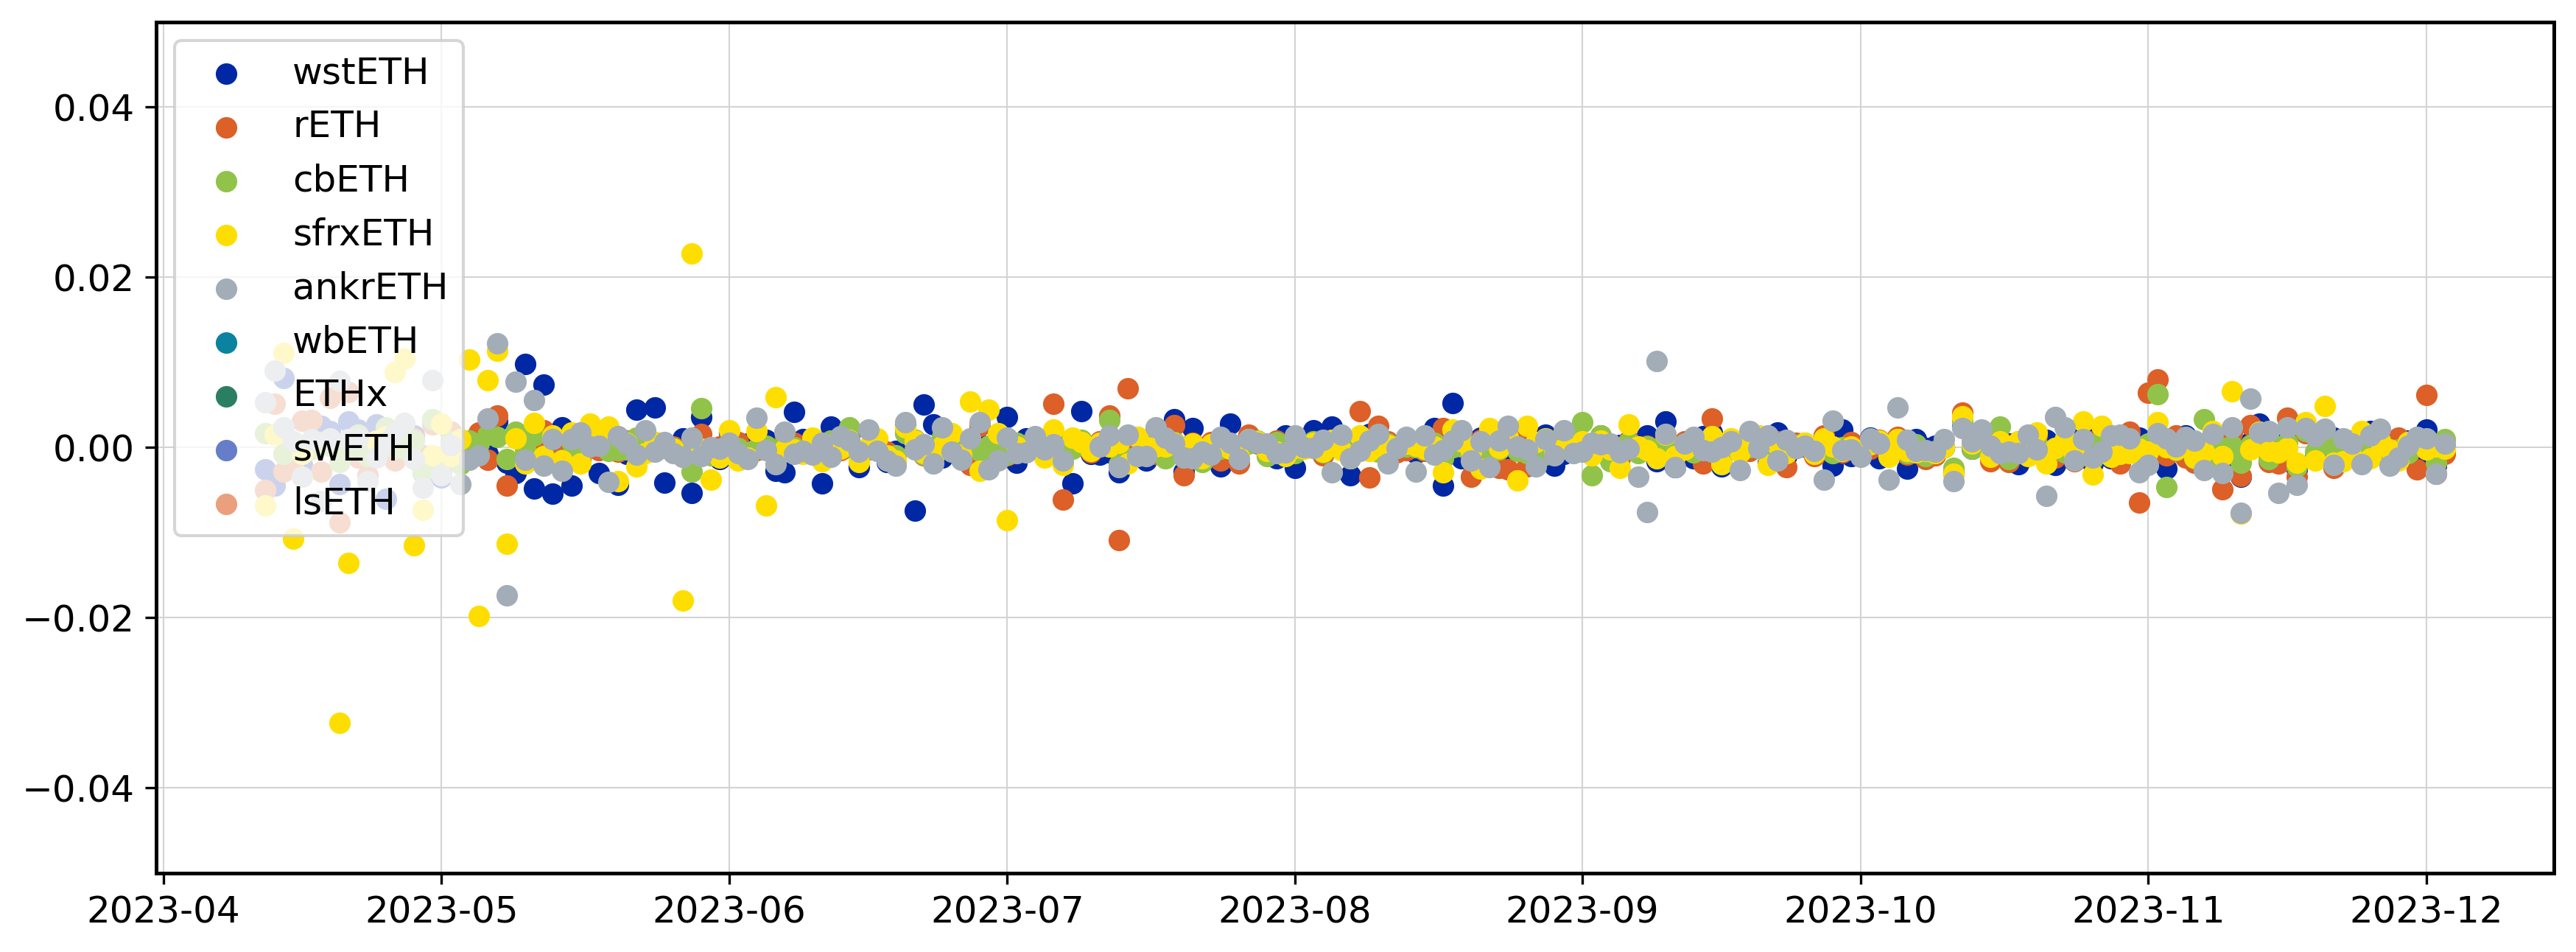} 
  \end{minipage} 
  \caption{Distribution of deviations for rebase-LSTs and reward-LSTs: The top row shows the differences between the market price of rebase-LSTs and the target value of 1 ETH, while the bottom row depicts the differences between the daily returns of reward-LSTs and the daily staking rate. The left column represents data since token inception, and the right column shows data after the Shanghai upgrade.}

  \label{fig:s_Ethereum}
\end{figure*}
